# Supplementary material for: ATTIQA: Generalizable Image Quality Feature Extractor using Attribute-aware Pretraining
Source: arXiv:2406.01020 source file (2024-10-05)
Supplement: Supplementary file 9 [file table_liqe.tex]

\begin{table}[htb!]
\label{t3}
\begin{center}
\caption{Performance comparison with LIQE.}
\resizebox{0.8\columnwidth}{!}
{
    \begin{tabular}{c|c||c|c|c|c|c|c||c|c|c}
    \toprule
    &\multirow{2}{*}{Methods} & \multicolumn{6}{c}{Seen Dataset} & \multicolumn{3}{c}{Unseen Dataset} \\
    &&LIVE & CSIQ & KADID & BID & LIVEC & KonIQ & TID & SPAQ & PIPAL\\
    \midrule
    SR& LIQE & 0.970 & \textbf{0.936} & \textbf{0.930} & 0.875 & \textbf{0.904} & 0.919 & \textbf{0.811} & 0.881 & 0.478 \\
    CC&ATTIQA & \textbf{0.974} & \textbf{0.936} & 0.923 & \textbf{0.891} & 0.901 & \textbf{0.920} & 0.796 & \textbf{0.891} & \textbf{0.521}\\
    \midrule
    PL&LIQE & 0.951 & 0.939 & \textbf{0.931} & 0.900 & 0.910 & 0.908 & - & - & - \\
    CC&ATTIQA & \textbf{0.977} & \textbf{0.950} & 0.927 & \textbf{0.918} & \textbf{0.917} & \textbf{0.932} & - & - & -\\
    \bottomrule
    \end{tabular}
}
\label{table:liqe}
\end{center}
\end{table}
